# Supplementary material for: Prompt Recovery for Image Generation Models: A Comparative Study of Discrete Optimizers
Source: arXiv:2408.06502 source file (2025-04-29)
Supplement: Supplementary file 1 [file appendix.tex]

\appendix

\section{Further Qualitative Examples}
\label{app:qual}

%     \begin{tabular}{c}
%         \input{figures/qualitative_results/example_1/table} \\
%         \\
%         \input{figures/qualitative_results/example_4/table} \\
%         \\
%         \input{figures/qualitative_results/example_6/table} \\
%     \end{tabular}

% \newpage
%     \begin{tabular}{c}
%         \input{figures/qualitative_results/example_7/table} \\
%         \\
%         \input{figures/qualitative_results/example_5/table} \\
%     \end{tabular}
